# Supplementary material for: Second Order Meanfield Approximation for calculating Dynamics in Au-Nanoparticle Networks
Source: arXiv:2402.12223 source file (2024-02-19)
Supplement: Supplementary file 1 [file appendix_algorithms.tex]

\label{appendix:B}
% ADAM and Gaussian algorithms, Pseudo-Code
\subsection{Discrete Gaussian Distribution}
To find the discrete Gaussian distribution in one dimension, the functional form
\begin{align}
    \rho(n) = \frac{1}{Z} \exp{\frac{(n - \mu)^2}{2\sigma^2}}
\end{align}
is taken at discrete $n \in \mathbb{Z}$. Since the underlying space is not $\mathbb{R}$, $\mu$ and $\sigma$ do not correspond to the mean and variance of this distribution. Rather, they are fit-parameters and must be optimised until:
\begin{align}
    \sum_{n} n \rho(n) &= \langle n \rangle \\
    \sum_{n} n^2 \rho(n) &= \langle n^2 \rangle
\end{align}
The idea of the algorithm is the heuristic of monotonically increasing relationships $\langle n \rangle(\mu)$ and $\Delta n(\sigma)$. Thus, the initial values for $\mu$ and $\sigma$ will be set to the target values $\langle n \rangle$ and $\Delta n$ and then optimised according to algorithm (\ref{alg:discrete_gaussian}).

\begin{algorithm}
    \caption{Finding Discrete Gaussian Probabilities}
    \label{alg:discrete_gaussian}
    \begin{algorithmic}
        \Require $\langle n \rangle$ and $\Delta n$
        \Ensure $\Delta n > 0$
        \State $\mu \gets \langle n \rangle$ \Comment{Initialise Parameters}
        \State $\sigma \gets \Delta n$
        \State $l = 0.9$ \Comment{Step Scaling}
        \For{i = 1; $i < 20$; i++} \Comment{or as many iterations as needed}
            \State p\_array = functional\_form($\mu$, $\sigma$) \Comment{Calculate probabilities on size 20 array}
            \State current\_mean, current\_var = calc\_moments(p\_array)

            \State $\mu \gets \mu + l (\langle n \rangle - \mathrm{current\_mean} )$ \Comment{Update using monotonicity heuristic}
            \State $\sigma \gets \sigma + l ((\Delta n)^2 - \mathrm{current\_var} )$
        \EndFor
        \State \Return functional\_form($\mu$, $\sigma$)
    \end{algorithmic}
\end{algorithm}

\subsection{ADAM-Optimisation Algorithm}
As the goal of some analysis is just focussing on the equilibrium state and indifferent to the preceding dynamics, the ADAM algorithm \cite{ADAM} used in this situation stores exponentially weighted averages of time derivatives of the first- and second-order moment. The ADAM algorithm is commonly used in Machine Learning to follow gradients of the cost function and is a state-of-the art choice because it can dampen artefactual oscillations created by the choice of a high step-size (which is desired because only the equilibrium is of interest) and rescale the derivatives entry-wise (independently for each island) to allow for faster and more stable convergence. The ADAM algorithm does not solve for the exact dynamics but helps to find its fixed point. The calculation and application of ADAM-steps is shown in (\ref{alg:adam}).

\begin{algorithm}
    \caption{ADAM-Algorithm to Find Equilibrium State}
    \label{alg:adam}
    \begin{algorithmic}
        \Require time derivative operator $\partial_t$
        \Require position in moment space $\vec{M}$
        \State $\beta_1 \gets 0.5$ \Comment{Hyperparameters}
        \State $\beta_2 \gets 0.999$
        \State $\vec{V_0} = 0$ \Comment{Initialise Averages}
        \State $\vec{V_1} = 0$
        \State $l = 0.1$ \Comment{Step Scaling}
        \While{not converged} \Comment{As many iterations as needed}
            \State $\vec{V_0} \gets \beta_1 \vec{V_0} + (1 - \beta_1) \cdot \partial_t \vec{M}$ \Comment{Update Averages}
            \State $\vec{V_1} \gets \beta_2 \vec{V_1} + (1 - \beta_2) \cdot (\partial_t \vec{M})^2$  (element wise)
            \State $\vec{M} \gets \vec{M} + l \cdot \vec{V_0} / \sqrt{\vec{V_1}} $ (element wise) \Comment{Update State}
        \EndWhile
        \State \Return $\vec{M}$
    \end{algorithmic}
\end{algorithm}
